# Supplementary material for: Geometric Neural Diffusion Processes
Source: arXiv:2307.05431 source file (2023-07-11)
Supplement: Supplementary file 1 [file consistency.tex]

\section{Consistency proof}
\emile{To remove?}

Here is a more generic version of Vincents proof (I think), although I am not 100\% convinced any more due to the prediction of the mean vector changing with difference combinations of inputs...

It also isn't clear to me where in the proof one assumes the consistency of the base distribution so I am not sure about this.

\begin{theorem}{Consistency of the reverse process}{}
  Assume the de-noising distribution is consistent, i.e. 
  \[q(y_t^0 | \y_{t+1}) = \int q(y_t^0, y_t^1 | \y_{t+1}) \mathrm{d}y_t^1\]
  Then the one step denoised distribution will be consistent.
\end{theorem}
\begin{proof}{}{}
  \begin{align}
    \int p(y_t^0, y_t^1) \mathrm{d} y_t^1 &= \int \int q(y_t^0, y_t^1 | y_{t+1}) p(y_{t+1}) \mathrm{d} y_{t+1} \mathrm{d} y_t^1  \\
    &= \int \int q(y_t^0, y_t^1 | y_{t+1}) \mathrm{d} y_t^1 p(y_{t+1}) \mathrm{d} y_{t+1} \\
    &= \underbrace{\int q(y_t^0 | y_{t+1}^{0,1}) p(y_{t+1}^{0,1}) \mathrm{d} y_{t+1}}_{\text{not the right def}}  \\
    \text{\textcolor{red}{wrong! }} &= p(y_t^0)\\
  \end{align}
\end{proof}

I think we need to show something subtly different.

The marginal distribution defined on \(x_0\) by our model is given by
\[ q_{x_0}(y_t^0) = \int p_{x_0}(y_T^0) \prod_{i=T-1}^t q_{x_0}(y_{i}^0 | y_{i+1}^0) \mathrm{d}y_{T:{t+1}}^0 \]

The marginal distribution defined on \(x_0, x_1\) by our model is given by
\[ q_{x_0, x_1}(y_t^0, y_t^1) = \int p_{x_0, x_1}(y_T^0, y_T^1) \prod_{i=T-1}^t q_{x_0, x_1}(y_{i}^0, y_i^1| y_{i+1}^0, y_{i+1}^1) \mathrm{d}y_{T:{t+1}}^{0,1} \]

We need to show that
\[q_{x_0}(y_t^0) = \int q_{x_0, x_1}(y_t^0, y_t^1) dy_t^1\]
We can assume that \(p_{x_0, x_1}(y_T^0, y_T^1)\) comes from a consistent stochastic process as we specify it.

We can also assume that \(q_{x_0, x_1}(y_{i}^0, y_i^1| y_{i+1}^0, y_{i+1}^1)\) is consistent, as we define that. However, I believe Vincents proof tacitly assumes these to be equal in the final line in order to arrive at its conclusion.

Crucially we know nothing however about the relationship between \(q_{x_0, x_1}(y_{i}^0| y_{i+1}^0, y_{i+1}^1)\) and \(q_{x_0}(y_{i}^0| y_{i+1}^0)\)
