# Supplementary material for: Geometric Neural Diffusion Processes
Source: arXiv:2307.05431 source file (2023-07-11)
Supplement: Supplementary file 2 [file architecture.tex]

\section{Equivariant score network}

\paragraph{SE(3)-transformer}
