# Supplementary material for: Geometric Neural Diffusion Processes
Source: arXiv:2307.05431 source file (2023-07-11)
Supplement: Supplementary file 3 [file discrete.tex]

% \section{Discrete process} \label{sec:discrete_process}
% %
% In the main section \cref{sec:diffusion_sp} we introduced a generative model for stochastic processes by designing an adequate continuous process (i.e.\ SDE).
% We then showed that the equivariance constraint amounts to constraining the score network.
% In the discrete setting where the process is defined via a markov kernel, we have a similar equivariance constraint:

% \begin{align}
%     p\left( \rho(g)\y_t |, \rho(g)\y_{t+1}, g \cdot \x, t \right) = p\left( \y_t |, \y_{t+1}, \x, t \right).
% \end{align}
