# Supplementary material for: Geometric Neural Diffusion Processes
Source: arXiv:2307.05431 source file (2023-07-11)
Supplement: Supplementary file 4 [file general_tensor_fields.tex]

\section{Generic tensor fields}
\label{app:generic_tensor}
