# Supplementary material for: Geometric Neural Diffusion Processes
Source: arXiv:2307.05431 source file (2023-07-11)
Supplement: Supplementary file 5 [file sampling.tex]

\section{Conditional sampling}
\label{sec:sampling}

\begin{proof}{}{}
Here we show that the noising-denoising corrector in \cref{alg:conditioning_renoising} is equivalent to the Langevin Dynamics corrector step of \cref{alg:conditioning_langevin}, and therefore that both algorithms approximately give the same conditional samples.
Specifically we aim to show that this following update
\begin{align}
 \begin{cases} \sbr{\textunderscore, \tilde{\v{y}}_{t-\gamma}^*} = \sbr{\red{\v{y}^c_t}, \tilde{\v{y}}_t^*} + \gamma \left\{ -\frac{1}{2} \left( m(\bar{\v{x}}) - \sbr{\red{\v{y}^c_t}, \tilde{\v{y}}_t^*} \right) + \mathrm{K}(\bar{\v{x}}, \bar{\v{x}}) \mathbf{s}_\theta(t, \bar{\v{x}}, \sbr{\red{\v{y}^c_t}, \tilde{\v{y}}_t^*}) \right\} + \sqrt{\gamma} \mathrm{K}(\bar{\v{x}}, \bar{\v{x}})^{1/2} Z \\
\tilde{\v{y}}_{t}^* = {\tilde{\v{y}}}_{t-\gamma}^* + \gamma \left\{ \frac{1}{2} \left( m({\v{x}^*}) - {\tilde{\v{y}}}_{t-\gamma}^* \right) \right\} + \sqrt{\gamma} \mathrm{K}({\v{x}^*}, {\v{x}^*})^{1/2} Z'
\end{cases}
\end{align}

is (approximately) equivalent to this Langevin dynamics step
\begin{align}
   \sbr{\textunderscore, \tilde{\v{y}}_{t-\gamma}^*} = \sbr{\textunderscore, \tilde{\v{y}}_{t-\gamma}^*} + \frac{\gamma}{2} \mathrm{K}(\bar{\v{x}}, \bar{\v{x}}) \mathbf{s}_\theta(t-\gamma, \bar{\v{x}}, \sbr{\red{\v{y}^c_{t-\gamma}}, \tilde{\v{y}}_{t-\gamma}^*}) + \sqrt{\gamma} \mathrm{K}(\bar{\v{x}}, \bar{\v{x}})^{1/2} Z .
\end{align}

\end{proof}
