# Supplementary material for: Geometric Neural Diffusion Processes
Source: arXiv:2307.05431 source file (2023-07-11)
Supplement: Supplementary file 6 [file score_parametrizations_old.tex]

Let's recall that we have $\Sigma_{t|0} = (1 - e^{-B(t)}) \mathbf{K}$, and denote by $\mathrm{L}_{t|0}$ and $\mathrm{S}$ respectively the Cholesky decomposition of $\Sigma_{t|0}=\mathrm{L}_{t|0} \mathrm{L}_{t|0}^\top$ and $\mathrm{K} = \mathrm{S} \mathrm{S}^\top$.

\emile{worth re reading \citet[Appendix B.6]{karras2022Elucidatinga} to get ideas of what should or shouldn't work}

The denoising score matching loss weighted by $\Lambda(t)$ is given by
\begin{align}
     \mathcal{L}(\theta)
     = \mathbb{E} \left[\| \mathrm{s}_\theta(t, \bfY_t) - \nabla_{{\bfY}_t} \log p_{t}({\bfY}_t| \bfY_0)\|_{\Lambda(t)}^2  \right]
\end{align}
where $\|x-y\|^2_\Lambda 
= (x-y)^\top \Lambda (x-y) 
% = (x-y)^\top \Lambda^{1/2} {\Lambda^{1/2}^}^\top (x-y) 
% = ({\Lambda^{1/2}}^\top x - {\Lambda^{1/2}}^\top y)^\top  ({\Lambda^{1/2}}^\top x-{\Lambda^{1/2}}^\top y) 
= \|{\Lambda^{1/2}}^\top x - {\Lambda^{1/2}}^\top y\|_2^2$.
% \vincent{Should there not be a ${\Lambda^{1/2}}^\top$ somewhere?}

\paragraph{No preconditioning:}
\begin{align}
\begin{cases}
h_\theta(t, \cdot) = \mathrm{s}_\theta(t, \cdot) \approx \nabla \log p_{t}(\cdot) \\
\mathrm{K} \mathrm{s}_\theta(t, \cdot) = \mathrm{K}~ h_\theta(t, \cdot)
\end{cases}
\end{align}
% \begin{align}
%     \nabla_{{\bfY}_t} \log p_{t}({\bfY}_t| \bfY_0) = - \mathrm{L}_{t|0}^{-\top} \epsilon
% \end{align}

\begin{align}
     \mathcal{L}(\theta) 
     % & = \mathbb{E}_t \left[ \lambda(t) ~\mathbb{E}_{\bfY_0,\bfY_t}~ \| \nabla_{{\bfY}_t} \log p_{t}({\bfY}_t| \bfY_0) - (- \mathrm{L}_{t|0}^{-\top} \epsilon )\|_2^2 \right]
     = \mathbb{E} \left[ \| s_\theta(t,\bfY_t) + \mathrm{L}_{t|0}^{-\top} \epsilon \|_{\Lambda(t)} ^2 \right].
\end{align}
Choosing $\Lambda(t) = \mathrm{L}_{t|0} \mathrm{L}_{t|0}^{\top}$ we have
\begin{align}
      \mathcal{L}(\theta) 
      &=\mathbb{E} \left[ \| s_\theta(t,\bfY_t) + \mathrm{L}_{t|0}^{-\top} \epsilon \|_{ \mathrm{L}_{t|0} \mathrm{L}_{t|0}^{\top}}^2 \right] \\
      &=\mathbb{E} \left[ \| \mathrm{L}_{t|0}^{\top} s_\theta(t,\bfY_t) + \epsilon \|_2^2 \right] \\
      &=\mathbb{E} \left[ \| (1 - e^{-B(t)})^{1/2} \mathrm{S}^\top s_\theta(t,\bfY_t) + \epsilon \|_2^2 \right].
\end{align}
\emile{this is actually unstable, why?}

\paragraph{$\mathrm{S}^\top$ preconditioning:}

\begin{align}
\begin{cases}
h_\theta^\mathrm{S}(t, \cdot) = \mathrm{S}^\top \mathrm{s}_\theta(t, \cdot) \approx \mathrm{S}^\top \nabla \log p_{t}(\cdot) \\
\mathrm{K} \mathrm{s}_\theta(t, \cdot) = \mathrm{S} \mathrm{S}^\top \mathrm{s}_\theta(t, \cdot) = \mathrm{S}~ h_\theta^\mathrm{S}t, \cdot)
\end{cases}
\end{align}

With the weighting $\Lambda(t) = \mathrm{L}_{t|0} \mathrm{L}_{t|0}^{\top}$ we have

\begin{align}
      \mathcal{L}(\theta)
      &=\mathbb{E} \left[ \| (1 - e^{-B(t)})^{1/2} ~h^{\mathrm{S}}_\theta(t,\bfY_t) + \epsilon \|_2^2 \right].
\end{align}

\emile{this is actually unstable, why?}

\paragraph{$\mathrm{K}$ preconditioning:}

\begin{align}
\begin{cases}
h_\theta^\mathrm{K}(t, \cdot) = \mathrm{K} \mathrm{s}_\theta(t, \cdot)  = \mathrm{K} \nabla \log p_{t}(\cdot) \\
\mathrm{K} \mathrm{s}_\theta(t, \cdot) = h_\theta^\mathrm{K}(t, \cdot)
\end{cases}
\end{align}

With the weighting $\Lambda(t) = (1 - e^{-B(t)}) ~\mathrm{K}^\top \mathrm{K}$ we have
\begin{align}
      \mathcal{L}(\theta) 
      &=\mathbb{E} \left[ \| s_\theta(t,\bfY_t) + \mathrm{L}_{t|0}^{-\top} \epsilon \|_{(1 - e^{-B(t)}) \mathrm{K}^\top \mathrm{K}}^2 \right] \\
      &=\mathbb{E} \left[ \| (1 - e^{-B(t)})^{1/2} \mathrm{K} s_\theta(t,\bfY_t) + \mathrm{K} \mathrm{L}_{t|0}^{-\top} \epsilon \|_2^2 \right] \\
      &=\mathbb{E} \left[ \| (1 - e^{-B(t)})^{1/2} h_\theta^\mathrm{K}(t,\bfY_t) + (1 - e^{-B(t)})^{1/2} \mathrm{S} \mathrm{S}^\top (1 - e^{-B(t)})^{-1/2} \mathrm{S}^{-\top} \epsilon \|_2^2 \right] \\
      &=\mathbb{E} \left[ \| (1 - e^{-B(t)})^{1/2} h_\theta^\mathrm{K}(t,\bfY_t) + \mathrm{S}\epsilon \|_2^2 \right].
\end{align}

\emile{this is actually works ok}

% \begin{align}
%      (\mathbf{Ks})_\theta(\bar{\bfY}_t, \x, t)
%     %  (\mathbf{\Sigma s})_\theta(\bar{\bfY}_t, \x, t)
%      &\approx \mathbf{K} \nabla_{\bar{\bfY}_t}  \log p_{T-t}(t, \x, \bar{\bfY}_t) \\
%      % &= -  \left(1 - e^{-\int_{s=0}^t \beta_s ds} \right)^{-1} (\bar{\bfY}_t - m_{t|0}) \\
%      &= -  \left(1 - e^{-\int_{s=0}^t \beta_s ds} \right)^{-1} \Sigma_{t|0}^{1/2} \epsilon
% \end{align}


\paragraph{predicting $\bfY_0$:}
We have $\nabla_{{\bfY}_t} \log p_{t}({\bfY}_t| \bfY_0) = - \Sigma_{t|0}^{-1} (\bfY_t - m_{t|0}) = - \Sigma_{t|0}^{-1} (\bfY_t - e^{-\frac{1}{2} B(t)} \bfY_0) $ since $ m_{t|0} = e^{-\frac{1}{2} B(t)} \bfY_0$.
% thus $e^{-\frac{1}{2} B(t)} \left( \Sigma_{t|0}^{-1} \nabla_{{\bfY}_t} \log p_{t}({\bfY}_t| \bfY_0) + \bfY_t \right) = \bfY_0$.
% thus $\mathrm{s}_\theta(t, \cdot) \approx - \Sigma_{t|0}^{-1} (\bfY_t - m_{t|0}) $.
%
\begin{align}
\begin{cases}
% h_\theta^{\mathrm{Y}_0}(t, \cdot) = e^{-\frac{1}{2} B(t)} \left( \Sigma_{t|0}^{-1}  \mathrm{s}_\theta(t, \cdot) + \bfY_t \right) \approx \bfY_0  \\
h_\theta^{\mathrm{y}_0}(t, \cdot) \approx \bfY_0  \\
% \mathrm{K} \mathrm{s}_\theta(t, \cdot) = - (1 - e^{-B(t)})^{-1/2}  \mathrm{S}~ h_\theta^{\mathrm{Y}_0}(t, \cdot)
\mathrm{K} \mathrm{s}_\theta(t, \cdot) 
= - \mathrm{K} \Sigma_{t|0}^{-1} (\bfY_t - e^{-\frac{1}{2} B(t)} h_\theta^{\mathrm{Y}_0}(t, \cdot))
= - (1 - e^{-B(t)})^{-1} (\bfY_t - e^{-\frac{1}{2} B(t)} h_\theta^{\mathrm{Y}_0}(t, \cdot))
\end{cases}
\end{align}

\begin{align}
      \mathcal{L}(\theta) 
      &=\mathbb{E} \left[ \| h^{\mathrm{y}_0}_\theta(t,\bfY_t) - \bfY_0 \|_2^2 \right].
\end{align}

\emile{this is actually works ok}
